# Supplementary material for: Temperature-dependent Optoelectronic Properties of Quasi-2D Colloidal Cadmium Selenide Nanoplatelets
Source: arXiv:1710.09260 ancillary file (2017-10-25)
Supplement: Supplementary file 1 [file Ancillary_document_-_Temperature-dependent_Optoelectronic_Properties_of_Quasi-2D_Colloidal_Cadmium_Selenide_Nanoplatelets.pdf]

# Temperature-dependent Optoelectronic Properties of Quasi-2D Colloidal Cadmium Selenide Nanoplatelets

[Ancillary document]

Sumanta Bose, Sushant Shendre, Zhigang Song, Vijay Kumar Sharma,  
 Dao Hua Zhang, Cuong Dang, Weijun Fan, Hilmi Volkan Demir

October 25, 2017

## S1 Transition matrix elements equations

Expressions for the transition matrix elements  $\mathcal{P}_{cv,i}$  along the  $x$ ,  $y$  and  $z$  directions are given below.

$$\begin{aligned} \mathcal{P}_{cv,x} = \frac{p_0}{\sqrt{2}} \sum_{n_x, n_y, n_z} & [(a_{v,n_x, n_y, n_z}^2 + a_{v,n_x, n_y, n_z}^4) a_{c,n_x, n_y, n_z}^{1*} \\ & + (a_{v,n_x, n_y, n_z}^6 + a_{v,n_x, n_y, n_z}^8) a_{c,n_x, n_y, n_z}^{5*} \\ & + (a_{c,n_x, n_y, n_z}^{2*} + a_{c,n_x, n_y, n_z}^{4*}) a_{v,n_x, n_y, n_z}^1 \\ & + (a_{c,n_x, n_y, n_z}^{6*} + a_{c,n_x, n_y, n_z}^{8*}) a_{v,n_x, n_y, n_z}^5] \end{aligned} \quad (\text{S1a})$$

$$\begin{aligned} \mathcal{P}_{cv,y} = \frac{ip_0}{\sqrt{2}} \sum_{n_x, n_y, n_z} & [(a_{v,n_x, n_y, n_z}^2 - a_{v,n_x, n_y, n_z}^4) a_{c,n_x, n_y, n_z}^{1*} \\ & + (a_{v,n_x, n_y, n_z}^6 - a_{v,n_x, n_y, n_z}^8) a_{c,n_x, n_y, n_z}^{5*} \\ & + (a_{c,n_x, n_y, n_z}^{2*} - a_{c,n_x, n_y, n_z}^{4*}) a_{v,n_x, n_y, n_z}^1 \\ & + (a_{c,n_x, n_y, n_z}^{6*} - a_{c,n_x, n_y, n_z}^{8*}) a_{v,n_x, n_y, n_z}^5] \end{aligned} \quad (\text{S1b})$$

$$\begin{aligned} \mathcal{P}_{cv,z} = p_0 \sum_{n_x, n_y, n_z} & [a_{v,n_x, n_y, n_z}^3 a_{c,n_x, n_y, n_z}^{1*} \\ & + a_{v,n_x, n_y, n_z}^7 a_{c,n_x, n_y, n_z}^{5*} + a_{c,n_x, n_y, n_z}^{3*} a_{v,n_x, n_y, n_z}^1 \\ & + a_{c,n_x, n_y, n_z}^{7*} a_{v,n_x, n_y, n_z}^5] \end{aligned} \quad (\text{S1c})$$

where  $p_0 = \hbar \sqrt{\frac{E_p}{2m_e^*}}$  and  $E_p$  is the Kane matrix element.  $a_{c,n_x, n_y, n_z}$  and  $a_{v,n_x, n_y, n_z}$  are the plane wave expanding coefficient.

## S2 Dimensions of CdSe NPLs

In Fig. 5 of the main article we have shown a TEM image of our synthesized 4 ML CdSe NPL ensemble population. The TEM image is taken at 200 kV using the JEOL JEM-2010 HR TEM machine. The resolution of this TEM machine is  $\sim 0.22$  nm. Our TEM images have been analyzed using ImageJ software. In the TEM image, Fig. A1 below, we can clearly see NPLs in two orientations (i) face view (laterally flat) (ii) edge view (vertically stacked). Average lateral dimension of the NPLs are found to be  $22 \text{ nm} \times 8 \text{ nm}$ . Then, by carefully inspecting the stacked (vertical) NPLs, it is observed that the thickness of NPLs is decreasing from top to bottom. This is only possible when the stacked NPLs are tilted/folded and not exactly vertical, which is a common phenomenon for NPLs, as also observed by several other groups (*Nat. Mater.*, 2011, 10, 936 and *Nano Lett.*, 2014, 14 (11), 6257). This is confirmed by observing different thickness on the top ( $2.6 \pm 0.1$  nm) and bottom ( $1.73 \pm 0.2$  nm) part of the same NPLs using ImageJ software. Also, the ligands surrounding the NPLs have a contrast in the TEM image, so the NPL boundary is not strictly discernible. For this reason, thickness information obtained from this image will not be exactly 4 ML (1.2 nm). Also, the resolution of our TEM machine is  $\sim 0.22$  nm which is comparable to the thickness of 1 ML (0.3 nm) of CdSe NPLs. Therefore, TEM data cannot be conclusively used to comment on the  $\sim 1.2$  nm thickness for the 4 ML thick CdSe NPLs.

CdSe Nanoplatelets TEM

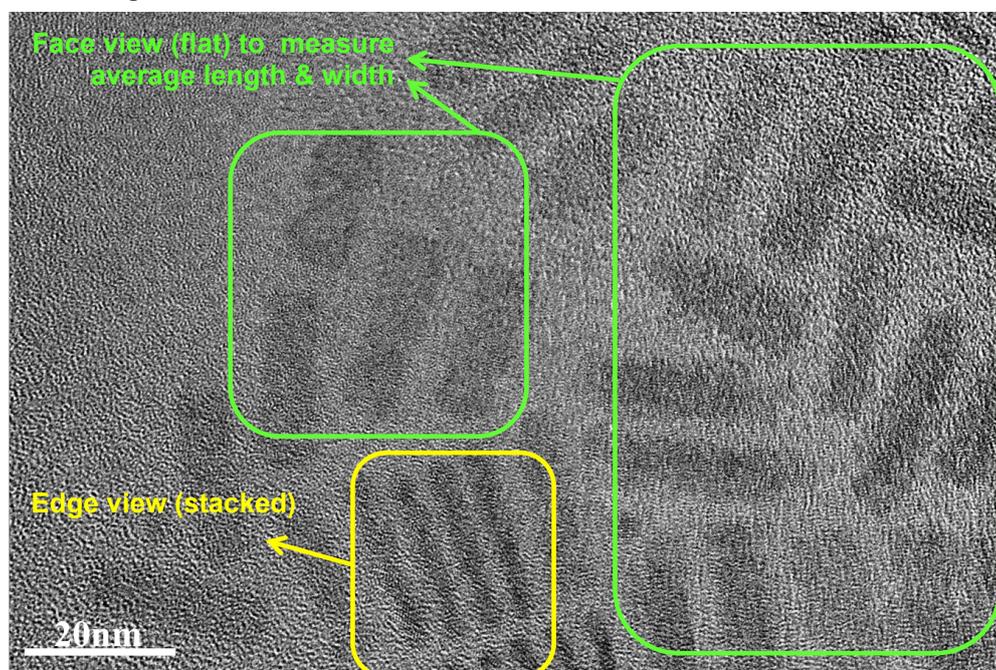

Figure S1: High-resolution TEM images of our synthesized 4 ML CdSe NPL population. The average NPL length and width were measured using ImageJ software from laterally flat lying NPLs and found to be  $22 \text{ nm} \times 8 \text{ nm}$ . From the edge view (stacked) NPLs, measurements show differing thicknesses at top and bottom, which is attributed to the tilting/folding of NPLs.

However, the optical properties of the CdSe NPLs with different thickness have very distinct features and are well established in the field of atomically flat NPLs. For 4 ML CdSe NPLs, the PL peak is observed at 512 nm and the absorption spectra have two distinct transition (light-hole 480 nm and heavy-hole 509 nm). Optical spectra results undoubtedly confirm that our CdSe NPLs are 4 ML (1.2 nm) thick. The quantized thickness of NPLs in ML can be converted to nm by computing  $\text{ML} \times (a/2)$  where  $a$  is the lattice constant of CdSe in nm. In our case, only TEM images cannot be directly used to make any claim that the CdSe NPLs are 4 ML. The claim is in conjunction with the optical spectra properties, which is well accepted in the field of NPLs.

### S3 Quasi Fermi energy levels and Fermi factor

Fig. S2 shows the conduction band (CB) and valence band (VB) quasi Fermi energy levels,  $E_{fc}$  and  $E_{fv}$  respectively, as a function of temperature for varying photogenerated carrier densities from 1 to  $5 \times 10^{19} \text{ cm}^{-3}$ . As the carrier density increases, the electrons and holes start to occupy higher CB and VB energy states, and thus their Fermi energy levels move farther away from the band edges. However, with increasing temperature, the both  $E_{fc}$  and  $E_{fv}$  approach the band edges. Thus, the quasi Fermi energy separation  $\Delta F = E_{fc} - E_{fv}$  decreases with temperature.

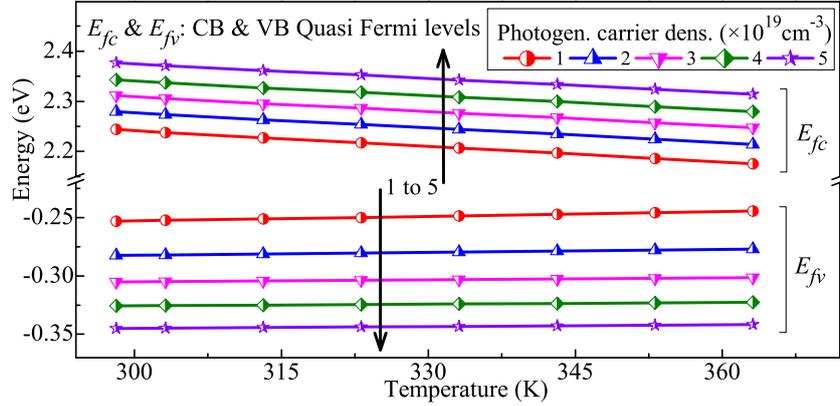

Figure S2: Quasi Fermi energy levels of the CB ( $E_{fc}$ ) and VB ( $E_{fv}$ ) as a function of temperature under varying photogenerated carrier densities. With increasing temperature,  $E_{fc}$  and  $E_{fv}$  approach each other and the Fermi energy separation decreases, as shown in Fig. 2b (in main paper) and Fig. S3.

Fig. S3 shows in contour form the variation of Fermi factor  $f_c(1 - f_v)$  for the E1–H1 transition and the Fermi energy separation  $\Delta F = E_{fc} - E_{fv}$  as a function of temperature and injection carrier concentration. With increasing carrier density both Fermi factor and  $\Delta F$  increase. However, temperature has the opposite effect. For a fixed density, a rise in temperature causes the fermions (electrons and holes) to get thermally excited and therefore the probability of occupying higher CB and VB energy states is increased; so the  $f_c$  falls, while  $f_v$  rises. Consequently the Fermi factor decreases with temperature. Also, the quasi Fermi levels of the CB and VB ( $E_{fc}$  and  $E_{fv}$ ) approach the band edges [Fig. S2], and therefore  $\Delta F$  falls.

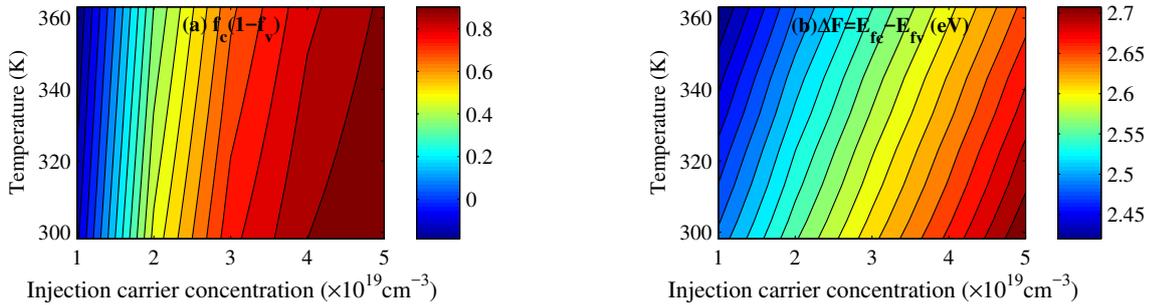

Figure S3: Contour plot of (a: *left*) Fermi factor  $f_c(1 - f_v)$  for the E1–H1 transition, and (b: *right*) Fermi energy separation  $\Delta F = E_{fc} - E_{fv}$  (eV) as a function of temperature and injection carrier concentration in 4 ML CdSe NPLs.

## S4 Interband Energy gap, Fermi factor and TME values

To understand the ongoing transition dynamics, we have shown in Fig. S4 the (a) transition energy, (b) Fermi factor for carrier density  $3 \times 10^{19} \text{ cm}^{-3}$ , (c) TE mode TME, and (d) TM mode TME for our 4 ML CdSe NPLs at  $30^\circ\text{C}$ , in contour form against the first ten CB and VB states. In Fig. 1b–d (main paper) we studied the electronic bandstructure showing the first ten CB and VB levels. Here, Fig. S4a shows the varying E–H transition energies, while Fig. S4b shows the corresponding Fermi factors for these transitions, the highest being the E1–H1 at 0.768. Only those with a positive value would contribute to the radiative recombination (see Eq. 7 and 8 in main paper). Finally, Fig. S4c–d shows the TE and TM mode TME values, giving an understanding of the allowed transitions with the highest possibilities. For the TE mode, the optical transition rule is followed, and the E1–H1 transition is the strongest with a TME value of 0.455. This is the heavy-hole dominated transition (see Fig. 1b in main paper). For the TM mode, however, the strongest is the E1–H9 transition, at 0.358, which is light-hole dominated. All of these correspond to the  $30^\circ\text{C}$ , and with a change in temperature, as discussed in the main paper (Fig. 1, Fig. 2 and Fig. 3), the transition energy, Fermi factor and the TME values decrease.

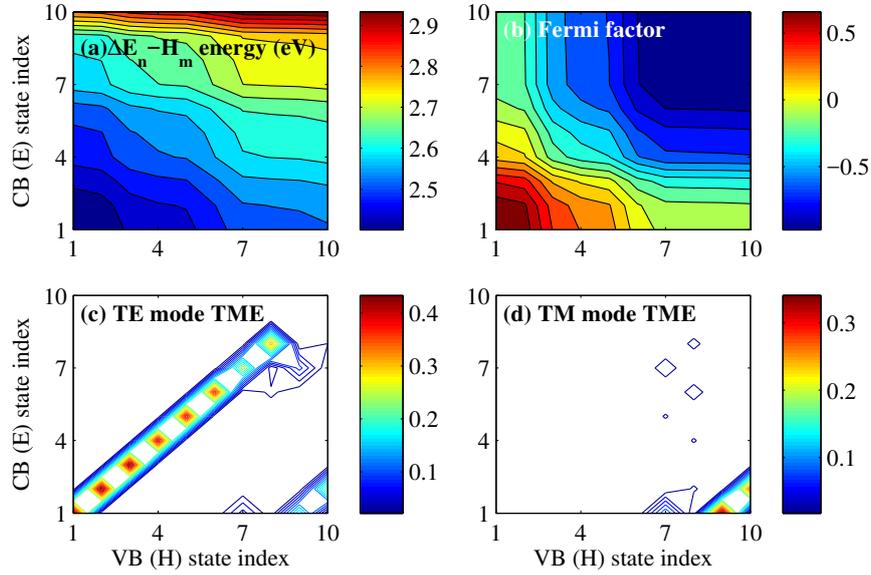

Figure S4: For 4 ML CdSe NPLs at  $30^\circ\text{C}$  (303.15 K), we have in contour form, the following: (a: *top left*) Transition energy between the first ten E and H states – the minimum (2.42 eV) occurs at  $\Delta\text{E}_{1-1}$ , (b: *top right*) Fermi Factor for an injection carrier density of  $3 \times 10^{19} \text{ cm}^{-3}$ ,  $\text{max} = 0.768$  at E1–H1 (c: *bottom left*) Transverse electric (TE) mode optical TME polarized in the  $x$ - $y$  plane, where E1–H1 is the strongest (0.455), and (d: *bottom right*) Transverse magnetic (TM) mode optical TME polarized along the  $z$  direction, where E1–H9 is the strongest (0.358). All contours are plotted against the first ten CB (E) and VB (H) state indices, and values specified in colorbars.

## S5 Comparison with published low-temperature result

Here we compare and validate our calculations and measurements with existing low-temperature results in literature. Fig. S5 shows the comparison of our calculated E1–H1 transition energy values (which matches with our experimental PL emission energy, Fig. 8 in main paper) with existing results from Achtstein *et al.* [*Nano Lett.* 2012 12 (6), 3151]. The red dot-line on the left frame is their experimental data for actual 4 ML CdSe NPLs at low temperature. The red plot in the right frame is our E1–H1 values from 303–363 K. The PL emission of  $512\pm 3$  nm ( $\sim 2.42$  nm) is from 4 ML NPLs, and the comparison with our results can be seen in the Fig. S5, showing the continuity in the PL emission energy.

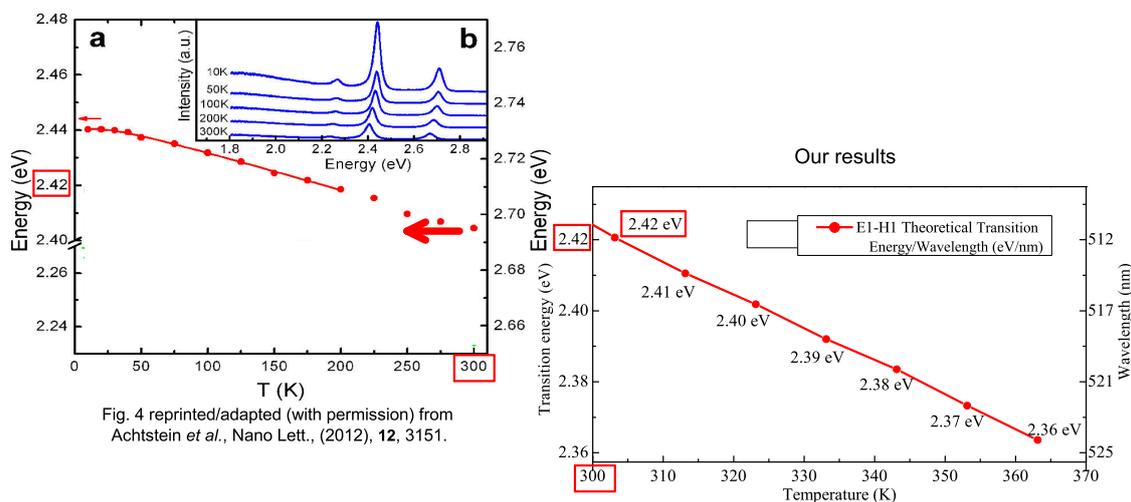

Figure S5: Comparison and extension of PL emission energy (by Achtstein *et al.*, [Reprinted (adapted) with permission from *Nano Lett.* 12 (6), 3151. Copyright (2012) American Chemical Society.] in the left frame) with our E1-H1 transition energy results in the right frame.

Also, as shown in Fig. S6, we have compared and extended our PL spectra at higher temperature ( $>RT$ ), with PL spectra at lower temperature ( $<RT$ ) as measured by Erdem *et al.* [*J. Phys. Chem. Lett.* 2016 7 (3), 548]. We have adjusted the  $x$ -axis range (2.3–2.55 eV) and  $y$ -axis range (0–2000) to ensure a correct superimposition of the results. The solid lines show the results of Erdem *et al.*, while the dotted lines show our result. There is a smooth continuity in the PL emission peak positions, PL linewidths and PL relative intensities. From Fig. S5 and S6, we believe that measurements and calculations done at lower temperature range would yield similar results for us.

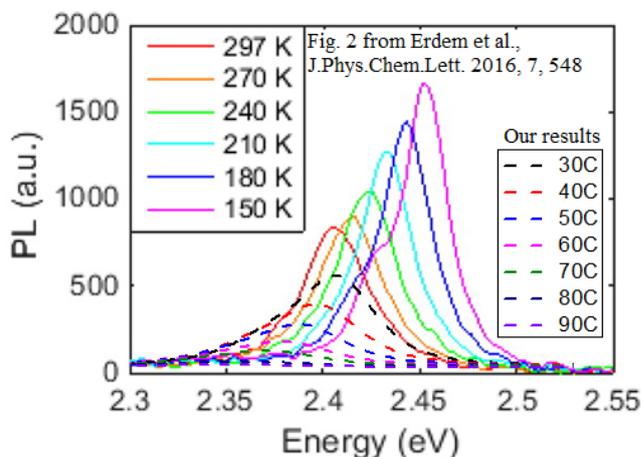

Figure S6: Comparison and extension of PL spectra (as measured by Erdem *et al.*, [Reprinted (adapted) with permission from *J. Phys. Chem. Lett.* 7 (3), 548. Copyright (2016) American Chemical Society.] in low temperature range shown by solid lines) with our PL spectra measurements at elevated temperature shown by dotted lines. There is a smooth continuity in the emission peak positions and the linewidths.

## S6 Fit of TRPL data

Fig. S7 shows the time-resolved photoluminescence (TRPL) emission spectrum for our 4 ML CdSe NPLs at 30°C, as shown in Fig. 6 (in the main paper). The red curve shows the fitting for the dual exponential decay path mechanism following the model  $I(t) = a_1 e^{-t/\tau_1} + a_2 e^{-t/\tau_2}$ , with PL decay lifetimes of  $\tau_1 = 0.34$  ns and  $\tau_2 = 2.27$  ns with 30% and 70% contribution respectively, leading to an average lifetime of 2.15 ns calculated using  $\tau_{\text{avg}} = (a_1 \tau_1^2 + a_2 \tau_2^2) / (a_1 \tau_1 + a_2 \tau_2)$ . The TRPL measurements were done with a Becker & Hickl DCS 120 confocal scanning FLIM system with an excitation laser of 375 nm. The system has temporal resolution of 200 ps. The blue line shows the instrument response function.

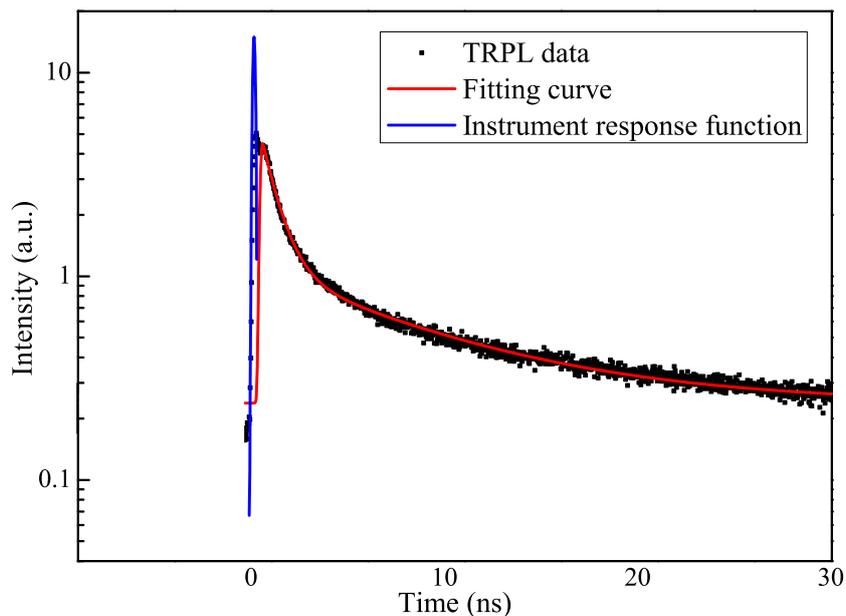

Figure S7: Time resolved Photoluminescence (TRPL) emission spectrum for 4 ML CdSe NPLs at 30°C (black dots), dual exponential decay fitting curve (red curve), and the instrument response function (blue line).

## S7 Database of experimental and theoretical results

Here we enlist, in Tables S1, S2 and S3, the experimental measurements (ascending and descending temperature) and theoretically calculated data for the PL emission energy, linewidth (and relaxation lifetime) and intensity, respectively, for varying temperature. For the experimental data, we have reported here the values obtained by Lorentzian fitting of the PL spectrum at every temperature. These correspond to the data plotted in Fig. 8 (in the main paper).

Table S1: Comparison of experimental (ascending and descending temperature) PL emission energy with theoretical E1–H1 transition energy for 4 ML CdSe NPLs at varying temperature.

| Temperature<br>(K) | Experimental emission energy (eV) [fitting data] |                        | Theoretical E1–H1<br>transition energy (eV) |
|--------------------|--------------------------------------------------|------------------------|---------------------------------------------|
|                    | Ascending Temperature                            | Descending Temperature |                                             |
| 298.15             | 2.42684                                          | 2.42484                | 2.42637                                     |
| 303.15             | 2.42113                                          | 2.41941                | 2.42066                                     |
| 313.15             | 2.41104                                          | 2.40961                | 2.41059                                     |
| 323.15             | 2.40229                                          | 2.40115                | 2.40188                                     |
| 333.15             | 2.39237                                          | 2.39152                | 2.39203                                     |
| 343.15             | 2.38071                                          | 2.38014                | 2.38352                                     |
| 353.15             | 2.37098                                          | 2.37069                | 2.37331                                     |
| 363.15             | 2.36133                                          | 2.36133                | 2.36362                                     |

Table S2: Experimental (ascending and descending temperature) PL linewidth and extracted intraband relaxation time  $\tau_{in}$  from ascending temperature data for 4 ML CdSe NPLs at varying temperature.

| Temperature<br>(K) | Experimental linewidth (meV) [fitting data] |                        | Extracted intraband<br>relaxation time $\tau_{in}$ (fs) |
|--------------------|---------------------------------------------|------------------------|---------------------------------------------------------|
|                    | Ascending Temperature                       | Descending Temperature |                                                         |
| 298.15             | 63.08751                                    | 64.64200               | 20.61268                                                |
| 303.15             | 65.25891                                    | 66.59133               | 19.96847                                                |
| 313.15             | 70.34078                                    | 71.45113               | 18.56839                                                |
| 323.15             | 73.67859                                    | 74.56687               | 17.76006                                                |
| 333.15             | 76.52492                                    | 77.19113               | 17.12800                                                |
| 343.15             | 80.74489                                    | 81.18903               | 16.25878                                                |
| 353.15             | 85.94988                                    | 86.17195               | 15.29642                                                |
| 363.15             | 88.00712                                    | 88.00712               | 14.95815                                                |

Table S3: Comparison of experimental (ascending and descending temperature) PL integrated intensity with theoretical relative intensity for 4 ML CdSe NPLs at varying temperature.

| Temperature<br>(K) | Experimental PL int. intensity ( $\times 10^5$ a.u.) [fitting data] |                        | Theoretical relative<br>PL intensity (a.u.) |
|--------------------|---------------------------------------------------------------------|------------------------|---------------------------------------------|
|                    | Ascending Temperature                                               | Descending Temperature |                                             |
| 298.15             | 13.4482                                                             | 1.3                    | 1                                           |
| 303.15             | 10.346                                                              | 1.2501                 | 0.808                                       |
| 313.15             | 7.6841                                                              | 1.1545                 | 0.62701                                     |
| 323.15             | 5.4731                                                              | 0.919                  | 0.4664                                      |
| 333.15             | 3.4325                                                              | 0.6402                 | 0.30493                                     |
| 343.15             | 2.2875                                                              | 0.3948                 | 0.195                                       |
| 353.15             | 0.838                                                               | 0.3469                 | 0.08051                                     |
| 363.15             | 0.4012                                                              | 0.4012                 | 0.0398                                      |
